# Supplementary material for: Auditing Representation-Induced Geometry in Acoustic-Emission Fracture Transients
Source: arXiv:2606.17061 source file (2026-09-01)
Supplement: Supplementary file 1 [file supplement.tex]

\documentclass[11pt]{article}

\usepackage[a4paper, margin=2.5cm]{geometry}
\usepackage{graphicx}
\usepackage{amsmath, amssymb}
\usepackage{hyperref}
\usepackage{caption}
\usepackage{subcaption}
\usepackage{booktabs}
\usepackage{pdfpages}
\usepackage{xcolor}

\title{Supplementary Material\\
A Transferable Morphology of Non-Gaussian Elastic Transients Across Physical Systems}

\author{Jose S\'anchez-Andreu\\
Aether Signal Intelligence}

\date{May 2026}

\begin{document}

\maketitle

\section*{Supplementary Atlas S1: Real-domain Grad-CAM transversal audit}

This supplementary atlas provides the full real-domain Grad-CAM audit for the frozen Aether encoder. The atlas includes per-sample attribution maps across source-domain interferometric examples, INSTANCE, IMS, OG1, OG3, and PRONOSTIA where available.

Each map is computed with respect to the frozen encoder latent-norm objective, using the same target layer and attribution protocol described in the main manuscript. These maps are interpreted as localization of encoder sensitivity to structured time-frequency regions, not as causal proof of identical physical mechanisms across domains.

\section*{Interpretation of the atlas}

The purpose of this atlas is to support the transversal Grad-CAM result shown in the main manuscript. The representative Figure 4 in the main paper summarizes selected examples across domains, while this supplementary atlas provides the broader per-sample audit.

The maps should be interpreted conservatively. They indicate where the frozen representation is most sensitive under the latent-norm Grad-CAM objective. They do not establish direct physical causality, source mechanism identity, or topological equivalence between domains.

\clearpage

\includepdf[
    pages=-,
    pagecommand={},
    width=\textwidth
]{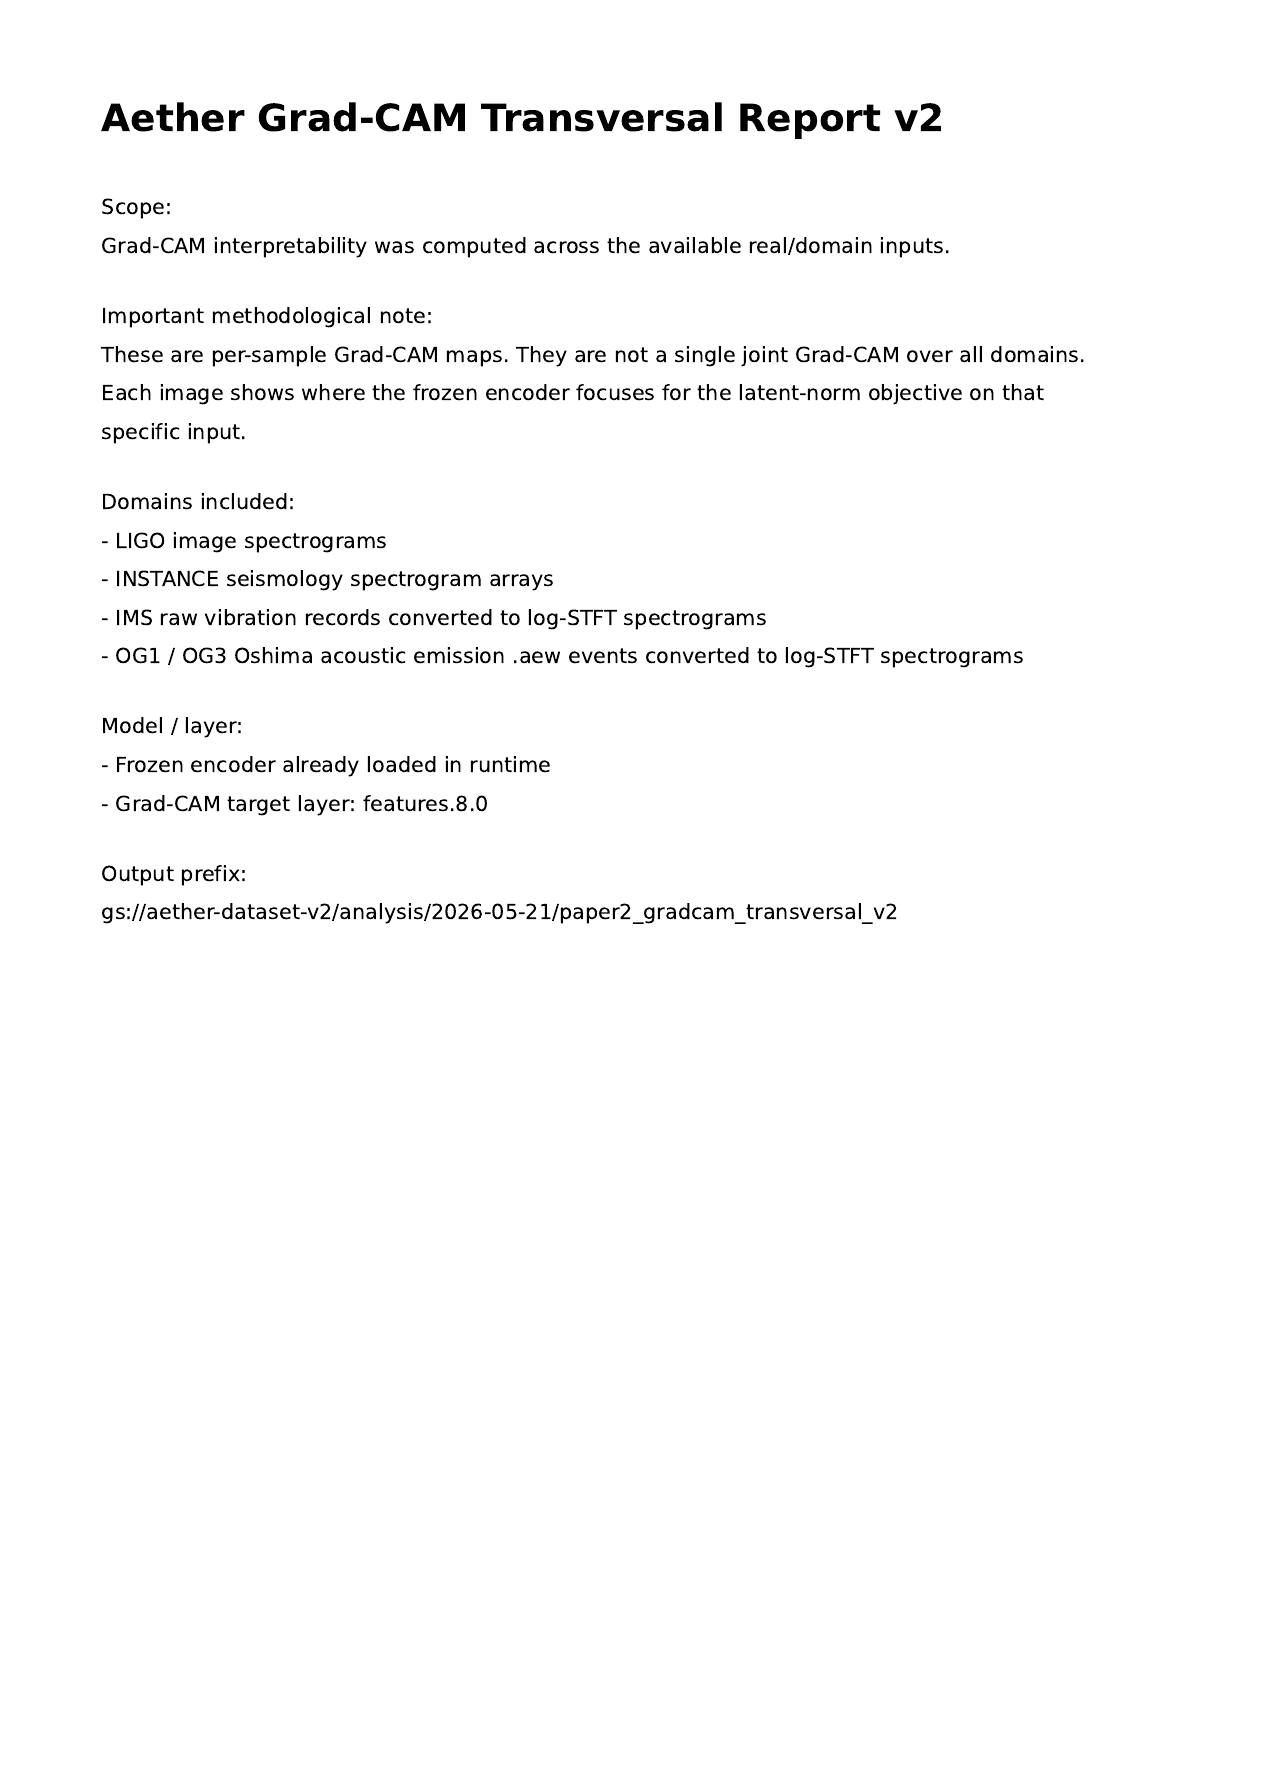}

\bibliographystyle{plain}
\bibliography{references}

\end{document}
